# Supplementary material for: MobRecon: Mobile-Friendly Hand Mesh Reconstruction from Monocular Image
Source: arXiv:2112.02753 source file (2022-03-31)
Supplement: Supplementary file 2 [file supplement_in_full.tex]

\section*{Supplementary Materials}
